# Supplementary material for: Mass and Eccentricity Constraints in the WASP-47 Planetary System from a Simultaneous Analysis of Radial Velocities & Transit Timing Variations
Source: arXiv:1612.04856 source file (2017-03-25)
Supplement: Supplementary file 1 [file appendix.tex]

\appendix
\section{First-Order Analytics of the Transit Timing Variations}
\label{sec:chopping}
For two planets near first order ($j:j-1$) mean motion resonance \cite{Lithwick12b}, give the following expression for $V$ and $V^\prime$, the  complex TTV amplitudes of the inner and outer planets respectively.

\begin{align}
    V        & = P \frac{\mu^\prime}{\pi j^{2/3} (j - 1)^{1/3} \Delta } 
                 \left(-f  - \frac{3}{2}\frac{\Zfreestar}{\Delta}\right) \label{eqn:v} \\
    V^\prime & = P^\prime \frac{\mu}{\pi j \Delta } 
                 \left(-g  + \frac{3}{2}\frac{\Zfreestar}{\Delta}\right) \label{eqn:vprime}, 
\end{align}
where $V$ is the complex TTV amplitude, $P$ is the average orbital period, $\Delta$ is the normalized distance to resonance given by

\begin{equation}
    \Delta = \frac{P^\prime}{P}\frac{j-1}{j} -1
\end{equation}    
and \Zfree is a linear combination of the free complex eccentricities of the the two planets given by
\begin{equation}
\Zfree = f \zfree + g \zfreeprime
\end{equation}
and $f$ and $g$ are order unity sums of Laplace coefficients. \Zfreestar is the complex conjugate of \Zfree.

For WASP-47, $P = P_b = 4.1592$~d, $P^{\prime} = P_d = 9.0316$~d, $\Delta = 0.0857$, $f = -1.010$, $g_{\mathrm{ext}} = 0.4284 - 1.17\Delta = 0.328 $. We consider a useful limiting case where $\Zfree / \Delta \ll g $ and $f$. The stability analysis by B15 found that $e < 0.06$ for all the planets.  Let us assume that the eccentricities of planets b and d are sufficiently small that $\Zfree / \Delta \lesssim g $ and $f$. Taking this limit, dividing Equation~\ref{eqn:v} by Equation~\ref{eqn:vprime}, and rearranging terms, we find:

\begin{align}
\frac{M_d}{M_b} & = \frac{g}{f}\left(\frac{j-1}{j}\right)^{1/3} \frac{P_d}{P_b} \frac{|V_b|}{|V_d|}\\
                   & \approx \frac{ 0.112}{0.328}
                     \left(\frac{1}{2}\right)^{1/3} 
                     \left( \frac{9.031\ \mathrm{d}}{4.159\ \mathrm{d}}\right)
                     \left( \frac{0.63\ \mathrm{min}}{7.5\ \mathrm{min}}\right) \\
                   & \approx 0.047
\end{align}
The \cite{Lithwick12b} formula loses accuracy as one moves away from first order MMR (as noted in \citet{Lithwick12b} and \citet{Deck2015_chopping}). This is because further away from resonance additional terms in the TTVs become comparable to the dominant terms associated with the resonance. For this system, with a period ratio of 2.17, these extra terms should be included. Using Equations (10)-(15) of Deck \& Agol 2015, the expression for the TTV amplitudes can be written as:
\begin{align}
    V &= {P \over 2\pi} \mu' f_1^{(2)}(\alpha) \nonumber \\
    V' & = {P' \over 2\pi} \mu f_2^{(1)}(\alpha)
\end{align}
where
\begin{align}
    \alpha & = \frac{a}{a'}, \nonumber \\
    f_1^{(2)}(\alpha) &= \alpha \frac{2 \beta D_\alpha b_{1/2}^{2}(\alpha)+(6+2\beta^2) b_{1/2}^{2}(\alpha) }{\beta^2 (1-\beta^2)},\\
    f_2^{(1)}(\alpha) &=  \bigg[(\kappa^2+3) b_{1/2}^{1}(\alpha)+2 \kappa (D_\alpha b_{1/2}^{1}(\alpha)+b_{1/2}^{1}(\alpha))\\
    &\qquad -\alpha^{-2} (\kappa^2-2\kappa+3) \bigg] \times \frac{1}{\kappa^2 (\kappa^2-1)},\\
    \beta &= 2(n-n')/n, \nonumber\\
    \kappa & = (n-n')/n',
\end{align}
and $D_\alpha$ is the derivative operator $\alpha \frac{\partial}{\partial \alpha}$, $n$ and $n'$ are the mean motions of the two planets, and $b_{1/2}^j(\alpha)$ is the usual Laplace coefficient.  For WASP-47 b and d, $\alpha = 0.596$, $f_1^{2} = -13.5$, and $f_2^{1} = 2.49$ (they are opposite in sign as the TTVs are anticorrelated).

We use a zeroth order formulae because we are considering the case where eccentricity effects are negligible, as argued above. In applying the formulae, we only include terms that would contribute a signal to the TTVs with a period equal to the ``super-period'' of the 2:1 near resonance, as those are the signal amplitudes we are measuring from the TTVs.
Evaluating these TTV expressions, using TTV amplitudes of 7.5 min and 0.63 min, we find  $M_d / M_b \approx 0.034$. 

Note that in the limit where eccentricity contributions are negligible, these formulae can be used to estimate the masses directly, and not just the mass ratio of the two planets. By doing so we find that $\mu' = 4.89\times10^{-5}$ and $\mu = 1.46\times10^{-3}$ (again using measured amplitudes of 7.5 and 0.63 minutes). Given a stellar mass of $\sim M_\odot$, this yields planet masses of 16.3 $M_\oplus$ and 487 $M_\oplus$, which are close to the answers we obtain in a full dynamical analysis of the TTVs alone.  

In reality, only the mass of planet d is well-determined from the TTVs, based on our N-body simulation.  This might be because we observed only one super-period of the TTV signal, and so the orbital p.  Likewise, the orbital periods of the planets would also be better determined if more than one super-period were observed, which would further contribute to a better mass determination. Carefully timed transit observations in the future might help resolve the amplitude and super-period of the TTV signal.
%{\bf not sure if you want to include this. but we can get the masses really simply from the formulae so might as well? That these are a bit high suggests that 0.75 and 7.5 min are too high as amplitudes. If I use Becker's measured TTV amplitude of 0.63 min, I get 16.3 earth masses. The HJ still has a mass that is too large, though. } 
